# Supplementary material for: Entire Four-Graviton EFT from the Duality Between Color and Kinematics
Source: arXiv:2601.09815 ancillary file (2026-07-01)
Supplement: Supplementary file 1 [file guideToAncFiles.pdf]

```

In[*]:= SetDirectory[NotebookDirectory[]];

In[*]:= gaugeData = Get["gaugeData.wl"];

In[*]:= gravityData = Get["gravityData.wl"];

In[*]:= Keys[gaugeData]
Out[*]:=
{4v, 2v2s, 3v1s}

```

---

## Some helper code

```

In[*]:= Attributes[dot] = {Orderless}

dot[-(a_), b_] := -dot[a, b]

dot[a_, (b_) + (c_)] := dot[a, b] + dot[a, c]

dot[c_, (b_) * (a_) ? NumberQ] := a * dot[b, c]
Out[*]:=
{Orderless}

In[*]:= extractType[data_, head_] := Union[Cases[data, head[___], {0, Infinity}]]

In[*]:= dotCofEqs[expr_] :=
  CoefficientArrays[expr, expr ~ extractType ~ dot] // Last // ArrayRules //
  (# == 0 & /@ Last /@ #) & // Union

polRules[multiplicity_] := {Table[dot[k[a], ep[k[a]]] -> 0, {a, Range[multiplicity]}], Table[ dot[myE,
Total[k /@ Range[multiplicity]]] == 0, {myE, ep /@ k /@ Range[multiplicity]}] /. dot[k[a_], ep[k[a_]]] -> 0
// Union // Reverse // Reduce // ToRules] // Flatten

getMomRules[myTrees_] := Module[{myLegs = myTrees /. Atree -> List /. -a_ -> a // Flatten // Union,
myEqns},
  myEqns = (myTrees /. Atree[a_] -> Table[dot[myLeg, Total@a] == 0, {myLeg, myLegs}]) ~ Join ~ (dot[#,
#] == 0 & /@ myLegs) // Flatten;
  Reduce[myEqns] // ToRules]

```

---

## Momentum and Pol Basis Rules

```

Out[*]:=
myMomRules = {dot[k[4], k[4]] -> 0, dot[k[3], k[3]] -> 0,
  dot[k[2], k[3]] -> -dot[k[2], k[4]] - dot[k[3], k[4]], dot[k[2], k[2]] -> 0,
  dot[k[1], k[4]] -> -dot[k[2], k[4]] - dot[k[3], k[4]], dot[k[1], k[3]] ->
  dot[k[2], k[4]], dot[k[1], k[2]] -> dot[k[3], k[4]], dot[k[1], k[1]] -> 0}

```

*Out[ ]:=*

```
myPolRules = {dot[ep[k[1]], k[1]] → 0,
  dot[ep[k[2]], k[2]] → 0, dot[ep[k[3]], k[3]] → 0, dot[ep[k[4]], k[4]] → 0,
  dot[ep[k[4]], k[1]] → -dot[ep[k[4]], k[2]] - dot[ep[k[4]], k[3]],
  dot[ep[k[3]], k[1]] → -dot[ep[k[3]], k[2]] - dot[ep[k[3]], k[4]],
  dot[ep[k[2]], k[1]] → -dot[ep[k[2]], k[3]] - dot[ep[k[2]], k[4]],
  dot[ep[k[1]], k[2]] → -dot[ep[k[1]], k[3]] - dot[ep[k[1]], k[4]]}
```

*In[ ]:=* basisRules = Dispatch@ (myMomRules ~Join~ myPolRules);

## Check Numerator Relations

### Setting up relations

```
In[ ]:= checkFFDressing[nsCand_, basisRules_] := Module[
  {ns = nsCand, nu = nsCand /. {k[4] → k[1], k[1] → k[4]},
   nt = nsCand /. {k[4] → k[2], k[2] → k[4]},
   notTrivialCheck, jacCheck, antiSymmCheck, isomorphicCheck},
  notTrivialCheck = (0 != (ns //. basisRules // Expand));
  If[! notTrivialCheck, Throw["Trivial Numerator!", nsCand]];
  jacCheck = (0 === (ns - nt - nu //. basisRules // Expand));
  If[! jacCheck, Throw["Bad Jacobi!", nsCand]];
  antiSymmCheck =
    (0 === (ns + (ns /. {k[1] → k[2], k[2] → k[1]}) //. basisRules // Expand)) &&
    (0 === (ns + (ns /. {k[3] → k[4], k[4] → k[3]}) //. basisRules // Expand));
  If[! antiSymmCheck, Throw[{"Not antisymmetric!", nsCand}]];
  isomorphicCheck =
    (0 === (ns - (ns /. Thread[Rule[k /@ Range[4], k /@ {3, 4, 1, 2}]])) //.
      basisRules // Expand));
  If[! isomorphicCheck, Throw[{"Not isomorphic!", nsCand}]];
  True]
```

```

In[*]:= checkDFDressing[nsCand_, basisRules_] := Module[
  {ns = nsCand, nu = nsCand /. {k[4] → k[1], k[1] → k[4]},
   nt = nsCand /. {k[4] → k[2], k[2] → k[4]},
   notTrivialCheck, jacCheck, antiSymmCheck, isomorphicCheck},
  notTrivialCheck = (0 != (ns //. basisRules // Expand));
  If[! notTrivialCheck, Throw["Trivial Numerator!", nsCand]];
  jacCheck = (0 === (ns + nt + nu //. basisRules // Expand));
  If[! jacCheck, Throw["Bad Jacobi!", nsCand]];
  antiSymmCheck =
    (0 === (ns - (ns /. {k[1] → k[2], k[2] → k[1]}) //. basisRules // Expand)) &&
    (0 === (ns + (ns /. {k[4] → k[3], k[3] → k[4]}) //. basisRules // Expand));
  If[! antiSymmCheck, Throw[{"Not antisymmetric!", nsCand}]];
  True]

In[*]:= checkDDDressing[nsCand_, basisRules_] := Module[
  {ns = nsCand, notTrivialCheck, symmCheck, isomorphicCheck},
  notTrivialCheck = (0 != (ns //. basisRules // Expand));
  If[! notTrivialCheck, Throw["Trivial Numerator!", nsCand]];

  symmCheck =
    (0 === (ns - (ns /. {k[1] → k[2], k[2] → k[1]}) //. basisRules // Expand)) &&
    (0 === (ns - (ns /. {k[3] → k[4], k[4] → k[3]}) //. basisRules // Expand));
  If[! symmCheck, Throw[{"Not symmetric!", nsCand}]];
  isomorphicCheck =
    (0 === (ns - (ns /. Thread[Rule[k/@Range[4], k/@{3, 4, 1, 2}]])) //.
     basisRules // Expand));
  If[! isomorphicCheck, Throw[{"Not isomorphic!", nsCand}]];
  True]

In[*]:= checkDressing["ff"][a_] := checkFFDressing[a, basisRules]
In[*]:= checkDressing["df"][a_] := checkDFDressing[a, basisRules]
In[*]:= checkDressing["dd"][a_] := checkDDDressing[a, basisRules]

```

## Verifying numerator relations

```
In[ ]:= type = "ff";
TableForm[ {#, Length[gaugeData["4v"][type][#]],
  And@@Table[ expr = Catch@checkDressing[type][myDressing],
    {myDressing, gaugeData["4v"][type][#] }]];
  TrueQ[expr] } & /@ Select[Keys[gaugeData["4v"][type]],
    Length[gaugeData["4v"][type][#]] > 0 &], TableHeadings →
  {{}, {"Mass Dimension", "# of "~~type~~" dressings", "Valid dressings"}}]
```

Out[ ]//TableForm=

| Mass Dimension | # of ff dressings | Valid dressings |
|----------------|-------------------|-----------------|
| 2              | 1                 | True            |
| 4              | 3                 | True            |
| 6              | 3                 | True            |
| 8              | 1                 | True            |

```
In[ ]:= type = "df";
TableForm[ {#, Length[gaugeData["4v"][type][#]],
  And@@Table[ expr = Catch@checkDressing[type][myDressing],
    {myDressing, gaugeData["4v"][type][#] }]];
  TrueQ[expr] } & /@ Select[Keys[gaugeData["4v"][type]],
    Length[gaugeData["4v"][type][#]] > 0 &], TableHeadings →
  {{}, {"Mass Dimension", "# of "~~type~~" dressings", "Valid dressings"}}]
```

Out[ ]//TableForm=

| Mass Dimension | # of df dressings | Valid dressings |
|----------------|-------------------|-----------------|
| 8              | 1                 | True            |
| 10             | 1                 | True            |
| 12             | 1                 | True            |

```
In[ ]:= type = "dd";
TableForm[ {#, Length[gaugeData["4v"][type][#]],
  And@@Table[ expr = Catch@checkDressing[type][myDressing],
    {myDressing, gaugeData["4v"][type][#] }]];
  TrueQ[expr] } & /@ Select[Keys[gaugeData["4v"][type]],
    Length[gaugeData["4v"][type][#]] > 0 &], TableHeadings →
  {{}, {"Mass Dimension", "# of "~~type~~" dressings", "Valid dressings"}}]
```

Out[ ]//TableForm=

| Mass Dimension | # of dd dressings | Valid dressings |
|----------------|-------------------|-----------------|
| 4              | 4                 | True            |
| 6              | 7                 | True            |
| 8              | 7                 | True            |
| 10             | 3                 | True            |

## Spanning games $ff \rightarrow d^{abcd} \subset dd$

```

In[ ]:= nffToDabcd[nsCand_] :=
  Module[{ns = nsCand, nt = nsCand /. Thread[Rule[k /@ Range[4], k /@ {4, 1, 2, 3}]]},
    nu = nsCand /. Thread[Rule[k /@ Range[4], k /@ {3, 1, 4, 2}]]},
    dot[k[2], k[3]] ns + dot[k[1], k[2]] nt ]

In[ ]:= type = "ff"; Print["Checking that d^{abcd} from ff passes dd checks"];
TableForm[ {#, Length[gaugeData["4v"][type][#]],
  And@@Table[ expr = Catch@checkDressing["dd"][myDressing],
    {myDressing, nffToDabcd /@ gaugeData["4v"][type][#] }]],
  TrueQ[expr] } & /@ Select[Keys[gaugeData["4v"][type]],
    Length[gaugeData["4v"][type][#]] > 0 &], TableHeadings ->
  {{}, {"Mass Dimension", "# of "~~type~~" dressings", "Valid dressings"}}]

Checking that d^{abcd} from ff passes dd checks

```

```

Out[ ]//TableForm=

```

|  | Mass Dimension | # of ff dressings | Valid dressings |
|--|----------------|-------------------|-----------------|
|  | 2              | 1                 | True            |
|  | 4              | 3                 | True            |
|  | 6              | 3                 | True            |
|  | 8              | 1                 | True            |

## check casting of ff to dabcd

We claim in the paper that all the  $d^{abcd}$  dressings are covered by  $n^{dd}$  dressings. Let's see that by casting the  $n^{ff}$  dressings to  $d^{abcd}$  dressings, and see if they're spanned by the  $n^{dd}$  dressings.

To case to  $d^4$  we use  $n^{d^4} = (n^{ff})_s t + (n^{ff})_t s$ . That's the `nffToDabcd[ns]` code. We now solve how to span that from the  $n^{dd}$  numerators  $\times$  permutation invariants.

```

In[ ]:= checkDabcdSpanning[nsCand_, basisRules_] := Module[
  {ns = nsCand, dABCD, correctOrder, guessDD,
   soln, validKeys = Keys@gaugeData["4v"]["dd"], sig2 = {},
   sig3 = {}, sig2Symb = {}, sig3Symb = {}, basis, basisSymb, rule},
  dABCD = nffToDabcd[ns] //. basisRules // Expand;
  correctOrder =
    Exponent[dABCD /. k[a_] => RandomReal[] k /. dot => Times /. ep[a_] => 1 /.
      k[a_] => RandomReal[] k, k];
  If[Length[Intersection[validKeys, {correctOrder - 4}]] > 0,
    sig2 = gaugeData["4v"]["dd"][correctOrder - 4] *
      (dot[k[1], k[2]]^2 + dot[k[2], k[3]]^2 + dot[k[1], k[3]]^2);
    sig2Symb =  $\sigma_2$  n[correctOrder - 4, #] & /@
      Range[Length[gaugeData["4v"]["dd"][correctOrder - 4]]];
  If[Length[Intersection[validKeys, {correctOrder - 6}]] > 0,
    sig3 = gaugeData["4v"]["dd"][correctOrder - 6] *
      (dot[k[1], k[2]]^3 + dot[k[2], k[3]]^3 + dot[k[1], k[3]]^3);
    sig3Symb =  $\sigma_3$  n[correctOrder - 6, #] & /@
      Range[Length[gaugeData["4v"]["dd"][correctOrder - 6]]];
  basis = Join[sig2, sig3, gaugeData["4v"]["dd"][correctOrder]];
  basisSymb = Join[sig2Symb, sig3Symb,
    n[correctOrder, #] & /@ Range[Length[gaugeData["4v"]["dd"][correctOrder]]];
  guessDD = MapIndexed[a[#2[[1]]] #1 &, basis] //. basisRules // Total;
  rule = dABCD - guessDD // dotCoefEqs // Reduce // ToRules;
  Total[MapIndexed[a[#2[[1]]] #1 &, basisSymb]] /. rule /. n[a_, b_] =>  $(n^a)_b$  ]

```

For example there's one MD 2 ff numerator.

```

In[ ]:= gaugeData["4v"]["ff"][2] // Length
Out[ ]:=
1

```

There's four gauge MD4 dd numerators

```

gaugeData["4v"]["dd"][4] // Length
Out[ ]:=
4

```

Can they span the MD 2 ff ->  $d^{\{abcd\}}$  ?

```

In[ ]:= checkDabcdSpanning[#, basisRules] & /@ gaugeData["4v"]["ff"][2] // TableForm
Out[ ]//TableForm=
 $n^4_1$ 

```

Yes, evidently we only need the first:

```
In[ ]:= XX gaugeData["4v"] ["dd"] [4] [[1] - YY nffToDabcd[gaugeData["4v"] ["ff"] [2] // First] //.
        basisRules // dotCoefEqs // Reduce
```

```
Out[ ]:=
XX == YY
```

There are 3 ff at mass dimension 4, which means 3 new  $d^{\{abcd\}}$  at mass dimension 6 -- are they spanned?

```
In[ ]:= gaugeData["4v"] ["ff"] [4] // Length
```

```
Out[ ]:=
3
```

```
In[ ]:= checkDabcdSpanning[#, basisRules] & /@ gaugeData["4v"] ["ff"] [4] // TableForm
```

```
Out[ ]//TableForm=

$$\begin{aligned} & n_1^6 + n_3^6 + n_7^6 \\ & - n_1^6 + n_6^6 \\ & n_4^6 + n_5^6 \end{aligned}$$

```

```
In[ ]:= gaugeData["4v"] ["ff"] [6] // Length
```

```
checkDabcdSpanning[#, basisRules] & /@ gaugeData["4v"] ["ff"] [6] // TableForm
```

```
Out[ ]:=
3
```

```
Out[ ]//TableForm=

$$\begin{aligned} & -3 n_1^8 + 2 n_2^8 + n_3^8 + n_4^8 - n_5^8 - n_6^8 + \frac{1}{2} n_4^4 \sigma_2 \\ & 3 n_1^8 - n_3^8 + n_4^8 + n_5^8 + n_6^8 + 2 n_7^8 + \frac{1}{2} n_3^4 \sigma_2 \\ & -n_2^8 - n_4^8 - n_7^8 + \frac{1}{2} n_2^4 \sigma_2 \end{aligned}$$

```

```
In[ ]:= gaugeData["4v"] ["ff"] [8] // Length
```

```
checkDabcdSpanning[#, basisRules] & /@ gaugeData["4v"] ["ff"] [8] // TableForm
```

```
Out[ ]:=
1
```

```
Out[ ]//TableForm=

$$\frac{1}{2} n_1^6 \sigma_2 + \frac{1}{2} n_3^6 \sigma_2 + \frac{1}{2} n_7^6 \sigma_2 + \frac{2}{3} n_1^4 \sigma_3 + \frac{2}{3} n_2^4 \sigma_3 + \frac{1}{3} n_3^4 \sigma_3 + \frac{1}{3} n_4^4 \sigma_3$$

```

## gravity spanning

```
In[ ]:= TableForm[ {#, Length@gravityData@#} & /@ Keys@gravityData,
  TableHeadings -> { {}, {"MD", "# G"} } ]
```

Out[ ]//TableForm=

|  | MD | # G |
|--|----|-----|
|  | 2  | 0   |
|  | 4  | 0   |
|  | 6  | 1   |
|  | 8  | 6   |
|  | 10 | 9   |
|  | 12 | 10  |
|  | 14 | 3   |
|  | 16 | 0   |

## Some helper functions

```
In[ ]:=  $\epsilon$  := ep
```

```
In[ ]:= getOrder[expr_] := Exponent[
  expr /. k[a_] -> RandomReal[] k /. dot -> Times /. ep[a_] -> 1 /. k[a_] -> RandomReal[] k, k]
```

```
In[ ]:= permListOfMD[n_] :=
  Table[If[IntegerQ[(n - 2 j) / 3],  $\sigma^2$ ^j  $\sigma^3$ ^((n - 2 j) / 3), {}], {j, 0, n / 2}] // Flatten
```

```
In[ ]:= gaugeData // Keys
```

Out[ ]:=

```
{4v, 2v2s, 3v1s}
```

```
In[ ]:= ffDC = Outer[Times, nfftToDabcd /@ Flatten[Values[gaugeData["4v"] ["ff"]]],
  nfftToDabcd /@ Flatten[Values[gaugeData["4v"] ["ff"]]]] // Flatten // Union //
  (# /. basisRules // FullSimplify) & // Sort[#, OrderedQ[getOrder /@ {#1, #2}] &] &;
```

```
In[ ]:= myFFDC = GroupBy[ffDC, getOrder];
```

```
In[ ]:= ddDC = Outer[Times, Flatten[Values[gaugeData["4v"] ["dd"]]],
  Flatten[Values[gaugeData["4v"] ["dd"]]]] // Flatten // Union //
  Sort[#, OrderedQ[getOrder /@ {#1, #2}] &] & //
  Sum[#, . Thread[Rule[k /@ Range[4], perm]],
  {perm, {k /@ Range[4], k /@ {1, 3, 4, 2}, k /@ {1, 4, 2, 3}}}] & /. basisRules;
```

```
In[ ]:= myDDDC = GroupBy[ddDC, getOrder];
```

```
In[ ]:= Keys[myFFDC]
```

Out[ ]:=

```
{8, 10, 12, 14, 16, 18, 20}
```

```
In[ ]:= Keys[myDDDC]
```

Out[ ]:=

```
{8, 10, 12, 14, 16, 18, 20}
```



```

In[*]:= allCoreDCMD = Union[Keys[myDDDC] ~Join~ Keys[myFFDC]]
Out[*]:=
{8, 10, 12, 14, 16, 18, 20}

In[*]:= mergeDC = Merge[{myFFDC, myDDDC}, Union[Flatten[#]] &];

In[*]:= ansatzForDC[targetMD_] := Module[{validMD = Select[allCoreDCMD, # ≤ targetMD &]},
  MapIndexed[a[#2[[1]]] #1 &,
    Table[ Outer[Times, permListOfMD[ (targetMD - vmd) / 2], mergeDC[vmd]] //
      Flatten // Union, {vmd, validMD}] // Flatten] // Total]

In[*]:= trRule = myTr[list__] := Module[{cntr = 0, mu},
  Times @@ Table[cntr++; myF /. lF[a_] := (k[a][mu[cntr]] × ε[k[a]][mu[cntr + 1]] -
    k[a][mu[cntr + 1]] × ε[k[a]][mu[cntr]]), {myF, list}] /. mu[cntr + 1] :=
    mu[1] // ExpandAll // (# /. a_[mu[i_]] × b_[mu[i_]] := dot[a, b]) &]
Out[*]:=
myTr[list__] := Module[{cntr = 0, mu},
  {#1 /. a_[mu[i_]] × b_[mu[i_]] := dot[a, b] &} [ExpandAll[Times @@ Table[cntr++;
    myF /. lF[a_] := k[a][mu[cntr]] × ε[k[a]][mu[cntr + 1]] - k[a][mu[cntr + 1]] ×
    ε[k[a]][mu[cntr]], {myF, list}] /. mu[cntr + 1] := mu[1]]]

In[*]:= quickPermInvts =
  Dispatch[{σ2 → dot[k[1], k[2]]^2 + dot[k[2], k[3]]^2 + dot[k[1], k[3]]^2,
    σ3 → dot[k[1], k[2]]^3 + dot[k[2], k[3]]^3 + dot[k[1], k[3]]^3} /. basisRules //
    FullSimplify]
Out[*]:=
Dispatch[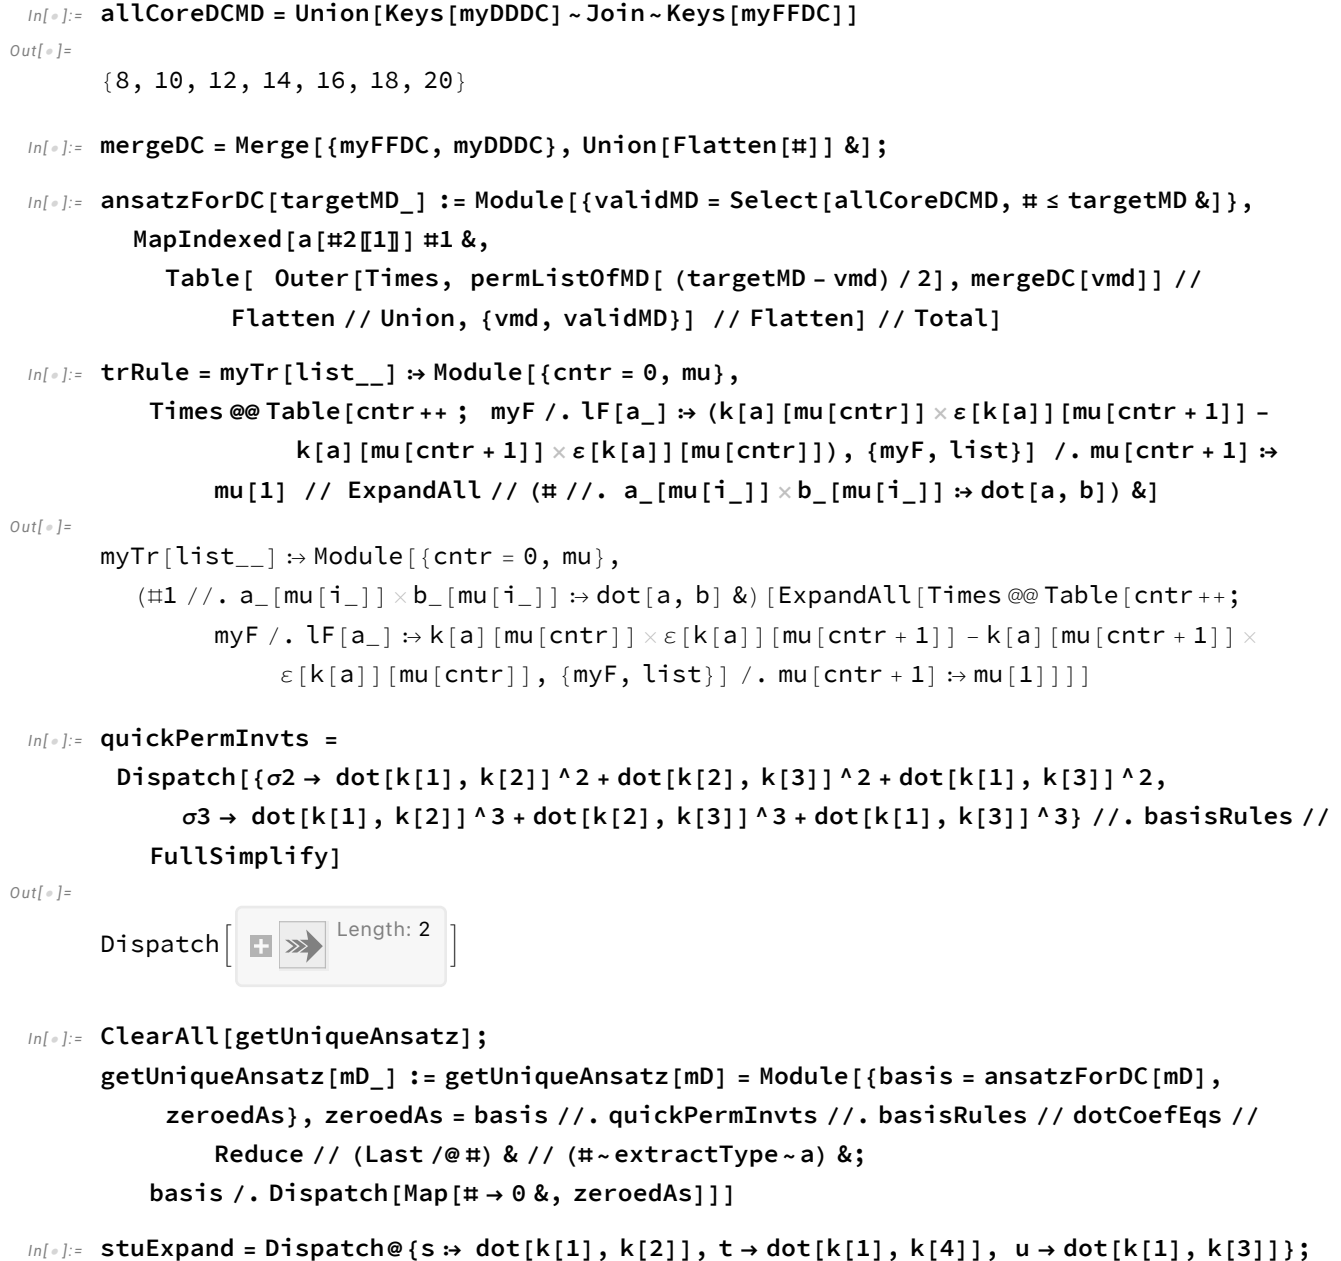]

In[*]:= ClearAll[getUniqueAnsatz];
getUniqueAnsatz[mD_] := getUniqueAnsatz[mD] = Module[{basis = ansatzForDC[mD],
  zeroedAs}, zeroedAs = basis /. quickPermInvts /. basisRules // dotCoefEqs //
  Reduce // (Last /@ #) & // (# ~extractType~ a) &;
  basis /. Dispatch[Map[# → 0 &, zeroedAs]]]

In[*]:= stuExpand = Dispatch@{s := dot[k[1], k[2]], t := dot[k[1], k[4]], u := dot[k[1], k[3]]};

```

## lovelock term MD6 from LEGO triple copy: $n^{\{d_4\}} n^{\{d_4\}} n^{\{d_4\}} + \text{perms}$

So what we're doing here to make the triple copy between 3 (vector  $\oplus$  scalar) blocks and summing over all permutations for graviton Bose symmetry.

```

In[*]:= checkPower[expr_] :=
  Exponent[(ExpandAll[expr] /. {k[a_] := RandomReal[], ep[a_] := 1}) /. dot := Times, k]

In[*]:= checkPower[lovelockTerm = gravityData[6][[1]]]
Out[*]:=
6

```

```
In[*]:= gA = (t u) myTr[{lF[1], lF[2]}] /. trRule /. stuExpand;
```

This satisfies  $d^4$  under all allowed exchanges ( $1 \leftrightarrow 2$ ) and ( $3 \leftrightarrow 4$ )

```
In[*]:= Table[gA - (gA /. perm),
  {perm, { {k[1] → k[2], k[2] → k[1]}, {k[3] → k[4], k[4] → k[3]},
    {k[1] → k[2], k[2] → k[1], k[3] → k[4], k[4] → k[3]}}} /. basisRules //
  Expand // Union // (# === {0}) &
```

```
Out[*]:=
True
```

```
In[*]:= gB = (s - t) (t - u) (s - u) myTr[{lF[2], lF[3], lF[4]}] /. trRule /. stuExpand;
```

This satisfies  $d^4$  under all allowed exchanges (perm(2,3,4))

```
In[*]:= Table[gB - (gB /. Thread[Rule[k /@ Range[2, 4], perm]]), {perm,
  Permutations[k /@ {2, 3, 4}]}] /. basisRules // Expand // Union // (# === {0}) &
```

```
Out[*]:=
True
```

```
In[*]:= gC = (s - t) (t - u) (s - u) myTr[{lF[1], lF[3], lF[4]}] /. trRule /. stuExpand;
```

This satisfies  $d^4$  under all allowed exchanges (perm(1,3,4))

```
In[*]:= Table[gC - (gC /. Thread[Rule[k /@ {1, 3, 4}, perm]]), {perm,
  Permutations[k /@ {1, 3, 4}]}] /. basisRules // Expand // Union // (# === {0}) &
```

```
Out[*]:=
True
```

```
In[*]:= tripleCopy = Sum[ gA gB gC /. Thread[Rule[k /@ Range[4], perm]],
  {perm, Permutations[k /@ Range[4]}}] /. basisRules;
```

```
In[*]:= tripleCopy //. quickPermInvts // getOrder
```

```
Out[*]:=
24
```

```
In[*]:= ((s - t) (t - u) (s - u) ) ^2 σ3 lovelockTerm /. quickPermInvts /. stuExpand // getOrder
```

```
Out[*]:=
24
```

```
In[*]:= spanningLoveLockTermEqns =
  ( getUniqueAnsatz[24] - (XXX tripleCopy - YYY ((s - t) (t - u) (s - u) ) ^2
    σ3 lovelockTerm) ) /. stuExpand //.
  quickPermInvts //. basisRules // Together // Numerator // dotCoefEqs;
```

```
In[*]:= goodSol = ExpandAll[spanningLoveLockTermEqns] // Reduce // ToRules
Out[*]= {a[194] → 0, a[191] → 0, a[190] → 0, a[91] → 0, a[90] → 0, a[87] → 0, a[86] → 0,
a[85] → 0, a[84] → 0, a[74] → - $\frac{a[75]}{6}$ , a[73] → 4 a[75], a[72] → - $\frac{2 a[75]}{3}$ ,
a[71] → a[75], a[70] → - $\frac{a[75]}{6}$ , a[69] → 4 a[75], a[68] → - $\frac{2 a[75]}{3}$ ,
a[63] → 0, a[62] → 0, a[59] → 0, a[58] → 0, a[55] → 0, a[54] → 0,
a[37] → 0, a[36] → 0, a[30] → 0, a[29] → 0, a[28] → 0, a[27] → 0, a[26] → 0,
a[24] → 0, a[23] → 0, a[16] → - $\frac{3 a[75]}{2}$ , a[15] →  $\frac{a[75]}{4}$ , a[10] → -2 a[75],
a[9] →  $\frac{a[75]}{3}$ , a[8] →  $\frac{a[75]}{4}$ , a[7] → - $\frac{a[75]}{24}$ , a[6] →  $\frac{a[75]}{2}$ , a[5] → - $\frac{a[75]}{12}$ ,
a[4] → - $\frac{a[75]}{2}$ , a[3] →  $\frac{a[75]}{12}$ , a[2] → 0, a[1] → 0, YYY → - $\frac{a[75]}{3}$ , XXX →  $\frac{a[75]}{24}$ }
```

## lovelock term MD6 from LEGO triple copy ( $n^{\{ff\}} n^{\{ff\}} n^{\{ff\}} n^{\{\pi, ff\}} / s$ )

What we're doing here to get the vector-scalar triple copy is:

- 1] composing composing two vector-scalar  $n^{\{ff\}}$  to make a  $n^{\{dd\}}$
- 2] composing the third vector-scalar  $n^{\{ff\}}$  with a pure scalar  $n^{\{ff\}}$  to make another  $n^{\{dd\}}$
- 3] We compose these  $n^{\{dd\}}$  together summing over all permutations to make the triple copy.

This is more involved because the BCJ solution for the 2-vectors and 2-scalars amplitude requires two different graph types. If the ext vectors are 1 and 4, then the s and u channel are graphs with a scalar propagator, and t-channel has a vector propagator. This means the graph dressings for  $n_s$  and  $n_u$  are related by relabeling, but  $n_t$  is functionally distinct (constrained by gauge invariance or Jacobi as usual). All that to say, is we need to specify channels individually before summing over permutations for Bose-statistics so the resulting gravitons from the triple copy can exchange. Note all cubic dressings are actually contacts in the gauge theory.

```
In[*]:= checkPower[expr_] :=
  Exponent[(ExpandAll[expr] /. {k[a_] := RandomReal[] k, ep[a_] := 1}) /. dot := Times, k]

In[*]:= checkPower[lovelockTerm = gravityData[6][[1]]]
Out[*]= 6

In[*]:= gAs =  $\sigma_3$  u myTr[{lF[1], lF[4]}] /. trRule /. stuExpand /. quickPermInvs;
gAu = gAs /. {k[2] → k[3], k[3] → k[2]};
gAt = gAs - gAu;
Residue[gAs / s /. stuExpand /. basisRules, {dot[k[3], k[4]], 0}]

Out[*]= 0
```

```

In[*]:= gBs = s myTr[{lF[2], lF[3], lF[4]]} /. trRule /.
    Dispatch@{s -> dot[k[1], k[2]], t -> dot[k[1], k[4]], u -> dot[k[1], k[3]]};
gBu = (gBs /. {k[2] -> k[3], k[3] -> k[2]});
gBt = (gBs /. {k[4] -> k[2], k[2] -> k[4]});
gBs - gBu - gBt //. basisRules // Expand

Out[*]=
0

In[*]:= gCs = s myTr[{lF[1], lF[2], lF[3]]} /. trRule /.
    Dispatch@{s -> dot[k[3], k[4]], t -> dot[k[1], k[4]], u -> dot[k[1], k[3]]};
gCu = (gCs /. {k[2] -> k[3], k[3] -> k[2]});
gCt = (gCs /. {k[1] -> k[3], k[3] -> k[1]});
gCs - gCu - gCt //. basisRules // Expand

Out[*]=
0

In[*]:= tripleCopy =
    Sum[ gAs gBs gCs (t - u) + gAt gBt gCt (s - u) + gAu gBu gCu (t - s) /. a[i_] -> c[i] /.
        Dispatch@{s -> dot[k[1], k[2]], t -> dot[k[2], k[3]], u -> dot[k[1], k[3]]} /.
        Thread[Rule[k /@ Range[4], perm]],
        {perm, Permutations[k /@ Range[4]]}] //. basisRules;

In[*]:= tripleCopy // getOrder

Out[*]=
22

In[*]:=  $\sigma_3^2 \sigma_2$  lovelockTerm /. quickPermInvts /. stuExpand // getOrder

Out[*]=
22

In[*]:= getUniqueAnsatz[22] /. quickPermInvts /. stuExpand // getOrder

Out[*]=
22

In[*]:= spanningLoveLockTermEqns =
    ( getUniqueAnsatz[22] - (XXX tripleCopy - YYY  $\sigma_3^2 \sigma_2$  lovelockTerm) /.
        stuExpand //. quickPermInvts //. basisRules ) // dotCoefEqns;

In[*]:= goodSol = ExpandAll[spanningLoveLockTermEqns] // Reduce // ToRules

Out[*]=

$$\left\{ \begin{aligned} &a[149] \rightarrow 0, a[146] \rightarrow 0, a[145] \rightarrow 0, a[92] \rightarrow 0, a[90] \rightarrow 0, a[89] \rightarrow 0, \\ &a[83] \rightarrow 4 a[84], a[82] \rightarrow a[84], a[81] \rightarrow 4 a[84], a[78] \rightarrow 0, a[76] \rightarrow 0, \\ &a[74] \rightarrow 0, a[41] \rightarrow 0, a[40] \rightarrow 0, a[39] \rightarrow 0, a[38] \rightarrow 0, a[27] \rightarrow 0, a[26] \rightarrow 0, \\ &a[25] \rightarrow 0, a[24] \rightarrow 0, a[23] \rightarrow 0, a[22] \rightarrow 0, a[21] \rightarrow 0, a[20] \rightarrow 0, a[19] \rightarrow 0, \\ &a[18] \rightarrow 0, a[15] \rightarrow 0, a[14] \rightarrow 0, a[13] \rightarrow 0, a[12] \rightarrow 0, a[8] \rightarrow -2 a[84], \\ &a[5] \rightarrow -2 a[84], a[4] \rightarrow 0, a[3] \rightarrow 0, a[2] \rightarrow 0, a[1] \rightarrow 0, YYY \rightarrow a[84], XXX \rightarrow -\frac{a[84]}{4} \end{aligned} \right\}$$


```

## MD $\geq$ 8 Terms from DoubleCopy

Note `getUniqueAnsatz[MD]` uses all the double-copies, ff and dd, then permutation invariants to build an ansatz at mass dimension MD. We see that they cover all the rest.

### MD 8 spanned

```
In[*]:= (# - getUniqueAnsatz[8] //. quickPermInvts //. basisRules // dotCoefEqs // Reduce //
        ToRules) & /@gravityData[8]

Out[*]=
{ {a[8] → 0, a[5] → 0, a[4] → 0, a[3] → 0, a[2] → 1, a[1] → 0},
  {a[8] → 0, a[5] → 1, a[4] → 0, a[3] → 0, a[2] → 0, a[1] → 0},
  {a[8] → 1, a[5] → 0, a[4] → 0, a[3] → 0, a[2] → 0, a[1] → 0},
  {a[8] → -1, a[5] → 2, a[4] → - $\frac{1}{2}$ , a[3] → -1, a[2] → 2, a[1] → 0},
  {a[8] →  $\frac{1}{2}$ , a[5] → 0, a[4] → 0, a[3] →  $\frac{1}{2}$ , a[2] → 0, a[1] →  $\frac{1}{2}$ },
  {a[8] → -4, a[5] → -4, a[4] → 1, a[3] → 0, a[2] → -4, a[1] → -1} }
```

### MD 10 spanned

```
In[*]:= (# - getUniqueAnsatz[10] //. quickPermInvts //. basisRules // dotCoefEqs // Reduce //
        ToRules) & /@gravityData[10]

Out[*]=
{ {a[15] → 0, a[14] → 0, a[8] → 0, a[7] → 0, a[6] → 1,
  a[5] → 1, a[4] → 0, a[2] → 0, a[1] → 0}, {a[15] →  $\frac{1}{2}$ , a[14] → 0,
  a[8] →  $\frac{1}{2}$ , a[7] → 0, a[6] → 1, a[5] → 1, a[4] → 0, a[2] → 0, a[1] → 0},
  {a[15] → -1, a[14] → 0, a[8] → -1, a[7] → 0, a[6] → -3, a[5] → -4, a[4] → 0,
  a[2] → 0, a[1] → 0}, {a[15] →  $\frac{1}{2}$ , a[14] → 0, a[8] →  $\frac{1}{2}$ , a[7] → -1,
  a[6] → 2, a[5] → 2, a[4] → 0, a[2] → 0, a[1] → 0}, {a[15] → 0, a[14] → 0,
  a[8] → 1, a[7] → 2, a[6] → 0, a[5] → 2, a[4] → 0, a[2] → 0, a[1] → 0},
  {a[15] → 0, a[14] → 0, a[8] → 0, a[7] → -1, a[6] → 0, a[5] → 0, a[4] → 0,
  a[2] → -1, a[1] → -1}, {a[15] → -1, a[14] → -1, a[8] → -3,
  a[7] → 0, a[6] → -4, a[5] → -7, a[4] → -1, a[2] → 0, a[1] → 0},
  {a[15] → 1, a[14] → 2, a[8] → 3, a[7] → 2, a[6] → 4, a[5] → 6,
  a[4] → 1, a[2] → 2, a[1] → 2}, {a[15] → -1, a[14] → 0, a[8] → -1,
  a[7] → 2, a[6] → -4, a[5] → -4, a[4] → 1, a[2] → 2, a[1] → 1} }
```

## MD12 spanned

```
In[ ]:= good12 = Select[ Range[Length[ gravityData[12]]],
  ( ( gravityData[12][[#]] - getUniqueAnsatz[12] ) //. quickPermInvts //. basisRules //
    dotCoefEqs // Reduce) != False & ]

Out[ ]:=
{1, 2, 3, 4, 5, 6, 7, 8, 9, 10}

In[ ]:= good12 === Range[Length[ gravityData[12]]]

Out[ ]:=
True
```

## MD 14 spanned

```
In[ ]:= good14 = Select[ Range[Length[ gravityData[14]]],
  ( ( gravityData[14][[#]] - getUniqueAnsatz[14] ) //. quickPermInvts //. basisRules //
    dotCoefEqs // Reduce) != False & ]

Out[ ]:=
{1, 2, 3}

good14 === Range[Length[ gravityData[14]]]

Out[ ]:=
True
```
